# Supplementary material for: Deep Burst Denoising
Source: arXiv:1712.05790 source file (2017-12-15)
Supplement: Supplementary file 2 [file sres_supmat_fig.tex]

\newcommand{\turnheightnew}{0.3\textwidth}

\resizebox{0.99\textwidth}{!}{\begin{tabular}{@{\hskip 1mm}c@{\hskip 1mm}c@{\hskip 1mm}c@{\hskip 1mm}c@{\hskip 1mm}c@{\hskip 1mm}c@{}}

Bicubic & SFSR (Ours) & MFSR (Ours) & Ground truth \\

% <left> <lower> <right> <upper>

\includegraphics[height=\turnheightnew, angle=90, trim=2cm 0cm 6cm 0cm, clip=true]{figures/sres4x_supmat/stab/images_live_photos_output_sr4x_26_n.jpg} &
\includegraphics[height=\turnheightnew, angle=90, trim=2cm 0cm 6cm 0cm, clip=true]{figures/sres4x_supmat/stab/images_live_photos_output_sr4x_26_s.jpg} &
\includegraphics[height=\turnheightnew, angle=90, trim=2cm 0cm 6cm 0cm, clip=true]{figures/sres4x_supmat/stab/images_live_photos_output_sr4x_26_m.jpg} &
\includegraphics[height=\turnheightnew, angle=90, trim=2cm 0cm 6cm 0cm, clip=true]{figures/sres4x_supmat/stab/images_live_photos_output_sr4x_26_g.jpg}\\

\includegraphics[height=\turnheightnew, trim=4cm 0cm 2cm 0cm, clip=true]{figures/sres4x_supmat/stab/images_live_photos_output_sr4x_50_n.jpg} &
\includegraphics[height=\turnheightnew, trim=4cm 0cm 2cm 0cm, clip=true]{figures/sres4x_supmat/stab/images_live_photos_output_sr4x_50_s.jpg} &
\includegraphics[height=\turnheightnew, trim=4cm 0cm 2cm 0cm, clip=true]{figures/sres4x_supmat/stab/images_live_photos_output_sr4x_50_m.jpg} &
\includegraphics[height=\turnheightnew, trim=4cm 0cm 2cm 0cm, clip=true]{figures/sres4x_supmat/stab/images_live_photos_output_sr4x_50_g.jpg}\\

\includegraphics[height=\turnheightnew, trim=6cm 0cm 0cm 0cm, clip=true]{figures/sres4x_supmat/stab/images_live_photos_output_sr4x_73_n.jpg} &
\includegraphics[height=\turnheightnew, trim=6cm 0cm 0cm 0cm, clip=true]{figures/sres4x_supmat/stab/images_live_photos_output_sr4x_73_s.jpg} &
\includegraphics[height=\turnheightnew, trim=6cm 0cm 0cm 0cm, clip=true]{figures/sres4x_supmat/stab/images_live_photos_output_sr4x_73_m.jpg} &
\includegraphics[height=\turnheightnew, trim=6cm 0cm 0cm 0cm, clip=true]{figures/sres4x_supmat/stab/images_live_photos_output_sr4x_73_g.jpg}\\

\includegraphics[height=\turnheightnew, trim=0cm 3cm 0cm 3cm, clip=true]{figures/sres4x_supmat/stab/images_live_photos_output_sr4x_31_n.jpg} &
\includegraphics[height=\turnheightnew, trim=0cm 3cm 0cm 2cm, clip=true]{figures/sres4x_supmat/stab/images_live_photos_output_sr4x_31_s.jpg} &
\includegraphics[height=\turnheightnew, trim=0cm 3cm 0cm 3cm, clip=true]{figures/sres4x_supmat/stab/images_live_photos_output_sr4x_31_m.jpg} &
\includegraphics[height=\turnheightnew, trim=0cm 3cm 0cm 3cm, clip=true]{figures/sres4x_supmat/stab/images_live_photos_output_sr4x_31_g.jpg}\\

\includegraphics[height=\turnheightnew, trim=4cm 0cm 2cm 0cm, clip=true]{figures/sres4x_supmat/stab/images_live_photos_output_sr4x_26_n.jpg} &
\includegraphics[height=\turnheightnew, trim=4cm 0cm 2cm 0cm, clip=true]{figures/sres4x_supmat/stab/images_live_photos_output_sr4x_26_s.jpg} &
\includegraphics[height=\turnheightnew, trim=4cm 0cm 2cm 0cm, clip=true]{figures/sres4x_supmat/stab/images_live_photos_output_sr4x_26_m.jpg} &
\includegraphics[height=\turnheightnew, trim=4cm 0cm 2cm 0cm, clip=true]{figures/sres4x_supmat/stab/images_live_photos_output_sr4x_26_g.jpg}\\

\end{tabular}}
